# Supplementary material for: The space weather around the exoplanet GJ 436b
Source: arXiv:2306.15391 source file (2023-06-27)
Supplement: Supplementary file 1 [file appendix_aline.tex]

\appendix
\section{Calculation of orbital trajectories}

\begin{figure}[b]
    \centering
    \includegraphics[width=.48\textwidth]{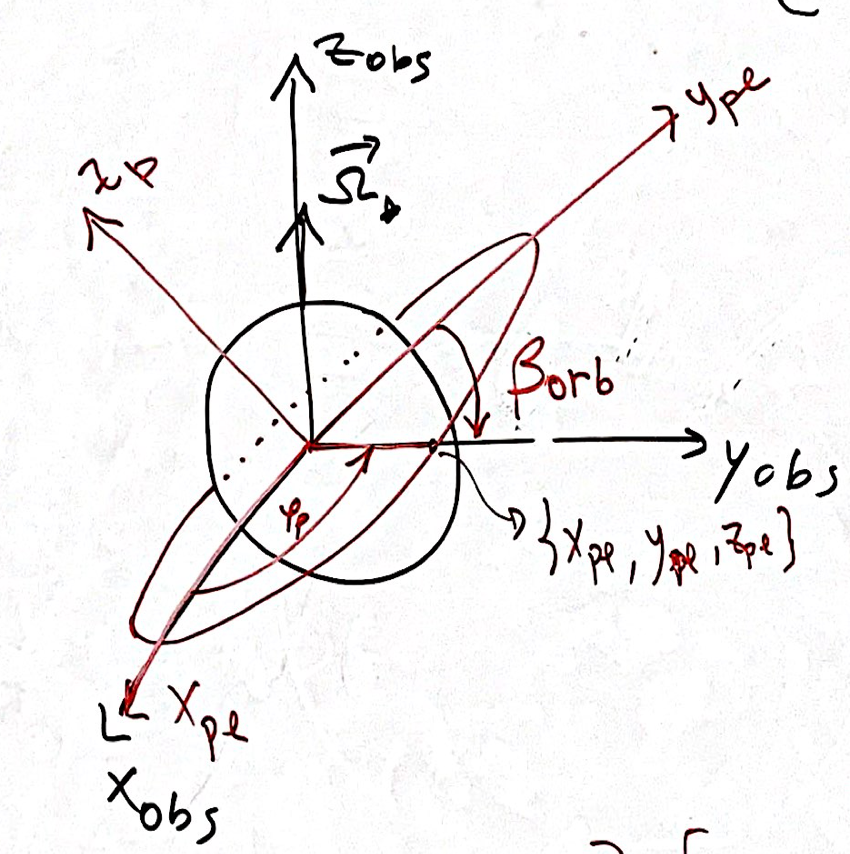} 
    \caption{Reference frames used in the coordinate transformation.}
    \label{fig.ref}%
\end{figure}

To calculate the orbital trajectories in the reference frame of the star, we compute two coordinate transformations: one from the orbital reference frame to the observer's frame, and another from the observer's frame to the stellar frame. These frames as illustrated in Figure \ref{fig.ref}.

We start from the orbital reference frame $\{x_{\rm pl}, y_{\rm pl}, z_{\rm pl}\} $, such that the $x_{\rm pl}y_{\rm pl}$-plane contains the orbit of the planet and the orbital axis is along $z_{\rm pl}$. The origin of this reference frame is  centred on the star. In this reference frame, the (circular) planetary motion is simply described as
\begin{equation}\label{eq.orb1}
\begin{bmatrix}
 x_{\rm pl} \\ y_{\rm pl}\\ z _{\rm pl}
\end{bmatrix}
= 
\begin{bmatrix}
R_{\rm orb} \cos \varphi_{\rm pl} \\
R_{\rm orb} \sin \varphi_{\rm pl} \\
0
\end{bmatrix} \, , 
\end{equation}
where the phase of the orbit $\varphi_{\rm pl} = \Omega_{\rm orb}t + \varphi_0$, with $t$ describing the time and $\Omega_{\rm orb}=2\pi/P_{\rm orb}$ the orbital rotation rate. Here, we assume a non-null initial phase $\varphi_0$, which we computed in Section 5 to find the location of GJ436b at zero phase of the ZDI maps. 

Now we take the observer's (inertial) reference frame $\{x_{\rm obs}, y_{\rm obs}, z_{\rm obs}\} $, whose origin is also  centred on the star, and  $z_{\rm obs}$ is aligned with the stellar rotation. We assume that $x_{\rm obs} \parallel x_{\rm pl}$. The angle between the orbital spin and the stellar spin axis is the true obliquity $\beta$, thus, the angle between $z_{\rm obs}$ and $z_{\rm pl}$ is also $\beta$. In this reference frame, the orbital motion of the planet is described as
\begin{equation}\label{eq.obs}
\begin{bmatrix}
 x_{\rm obs} \\ y_{\rm obs}\\ z _{\rm obs}
\end{bmatrix}
= 
\begin{bmatrix}
1 & 0& 0 \\
0 & \cos \beta & \sin \beta \\
0 & -\sin \beta & \cos \beta
\end{bmatrix}
\begin{bmatrix}
x_{\rm pl} \\ y_{\rm pl}\\ z _{\rm pl}
\end{bmatrix} \, ,
\end{equation}
where we performed an anticlockwise rotation around the axis $x_{\rm obs} \equiv x_{\rm pl}$ by an angle $\beta$.

The reference frame co-rotating with the star $\{x_\star, y_\star, z_\star\} $ is also centred on the star, with the stellar spin axis along $z_\star$, which is parallel to $z _{\rm obs}$. To transform from the observer's reference frame to the stellar co-rotating frame, we perform a clockwise rotation around the axis $ z_\star\equiv z_{\rm obs} $ by an angle $\Omega_\star t$
\begin{equation}\label{eq.star}
\begin{bmatrix}
 x_\star \\ y_\star \\ z_\star
\end{bmatrix}
= 
\begin{bmatrix}
\cos (\Omega_\star t) & -\sin (\Omega_\star t) &0\\
 \sin (\Omega_\star t) & \cos (\Omega_\star t) &0\\
0 & 0& 1 
\end{bmatrix}
\begin{bmatrix}
 x_{\rm obs} \\ y_{\rm obs}\\ z _{\rm obs}
\end{bmatrix} \, .
\end{equation}

Therefore, to derive the orbital path of the planet in the reference frame of the star, we use (\ref{eq.orb1}) and (\ref{eq.obs}) into (\ref{eq.star}), thus obtaining
% %
% \begin{equation}\label{eq.final}
% \begin{bmatrix}
%  x_\star \\ y_\star \\ z_\star
% \end{bmatrix}
% = 
% \begin{bmatrix}
% \cos (\Omega_\star t) & -\sin (\Omega_\star t) &0\\
%  \sin (\Omega_\star t) & \cos (\Omega_\star t) &0\\
% 0 & 0& 1 
% \end{bmatrix}
% \begin{bmatrix}
% 1 & 0& 0 \\
% 0 & \cos \beta & \sin \beta \\
% 0 & -\sin \beta & \cos \beta
% \end{bmatrix}
% \begin{bmatrix}
% R_{\rm orb} \cos \varphi_{\rm pl} \\
% R_{\rm orb} \sin \varphi_{\rm pl} \\
% 0
% \end{bmatrix} \, , 
% \end{equation}
%%
%\begin{equation}\label{eq.final}
%\begin{bmatrix}
% x_\star \\ y_\star \\ z_\star
%\end{bmatrix}
%= 
%\begin{bmatrix}
%\cos (\Omega_\star t) & -\sin (\Omega_\star t)  \cos \beta&-\sin (\Omega_\star t) \sin \beta\\
% \sin (\Omega_\star t) & \cos (\Omega_\star t)\cos \beta &\cos (\Omega_\star t)\sin \beta\\
%0 & -\sin\beta& \cos \beta
%\end{bmatrix}
%\begin{bmatrix}
%R_{\rm orb} \cos \varphi_{\rm pl} \\
%R_{\rm orb} \sin \varphi_{\rm pl} \\
%0
%\end{bmatrix} \, , 
%\end{equation}
%
%%
%\begin{equation}\label{eq.final}
%\begin{bmatrix}
% x_\star \\ y_\star \\ z_\star
%\end{bmatrix}
%= 
%\begin{bmatrix}
%\cos (\Omega_\star t)R_{\rm orb} \sin \varphi_{\rm pl}   -\sin (\Omega_\star t)  \cos \beta R_{\rm orb} \sin \varphi_{\rm pl}  \\
% \sin (\Omega_\star t)R_{\rm orb} \cos \varphi_{\rm pl} + \cos (\Omega_\star t)\cos \beta R_{\rm orb} \sin \varphi_{\rm pl}  \\
%-\sin\beta R_{\rm orb} \sin \varphi_{\rm pl}
%\end{bmatrix}
%\end{equation}
%
\begin{equation}\label{eq.finalx}
\frac{ x_\star}{R_{\rm orb} }= \cos (\Omega_{\rm orb}t + \varphi_0) \cos (\Omega_\star t)    - \sin (\Omega_{\rm orb}t + \varphi_0) \sin (\Omega_\star t)  \cos \beta 
\end{equation}
\begin{equation}\label{eq.finaly}
\frac{y_\star}{R_{\rm orb} } = \cos (\Omega_{\rm orb}t + \varphi_0) \sin (\Omega_\star t)  + \sin (\Omega_{\rm orb}t + \varphi_0) \cos (\Omega_\star t) \cos \beta  
\end{equation}
\begin{equation}\label{eq.finalz}
\frac{ z_\star}{R_{\rm orb} }= -\sin (\Omega_{\rm orb}t + \varphi_0) \sin \beta  \, .
\end{equation}
IIn the case of aligned systems, $\beta=0$ and we have
\begin{eqnarray}
{ x_\star}= R_{\rm orb}\cos (\Omega_{\rm orb}t + \varphi_0+\Omega_\star t) \\
{y_\star} = R_{\rm orb}\sin (\Omega_{\rm orb}t + \varphi_0 + \Omega_\star t) \\
{ z_\star}=0 \, .
\end{eqnarray}
I.e., in aligned systems, the planet re-encounters the same stellar wind property once every $2 \pi /(\Omega_{\rm orb}+\Omega_{\star})$.
